# Supplementary material for: Domain Game: Disentangle Anatomical Feature for Single Domain Generalized Segmentation
Source: arXiv:2406.02125 source file (2024-06-04)
Supplement: Supplementary file 1 [file supp.tex]

% \maketitle      
% \newpage

% \begin{center}
%  \Large  % Large
% \textbf{Domain Game: Disentangle Diagnostic Feature for Single Domain Generalised Segmentation} \\
% \vspace{0.3cm}
% \large 
% (Supplymentary Material)
% \end{center}

% \begin{center}
% \large
% \end{center}

% Reset the Section and using alphabet
% \setcounter{section}{0}
% \renewcommand{\thesection}{\Alph{section}}
% \thispagestyle{empty}

% \section{Experiments Details}
% \thispagestyle{empty}

% \subsection{{Metrics.}}
% \textbf{Dice Coefficient}:
% Dice coefficient is often used to measure the similarity between two sets. It is computed using the formula:

  % For brain tumor segmentation, our objective is to adapt segmentation models to accurately identify both
% due to its superior capability in delineating tumor morphology.
% This sequence is

% The brain tumor task segmentation distinguishes various glioma sub-regions: all portions of the necrotic tumor core (NTC $-$ label 1),  and the enhancing tumor (ET $-$ label 2). Clinically, ET regions on post-gadolinium T1-weighted (T1Gd) images are a frequent imaging characteristic for diagnosing gliomas \cite{kazerooni2023brain}, prompting us to use T1Gd images for training and validation purposes.

% Table~\ref{tab1}
% \noindent\textbf{Reference Note:}{ The reference list is included in the main paper.  }

% \bibliographystyle{splncs04}

% \bibliography{mybibliography}

% \bibliographystyle{splncs04}
% \bibliography{mybibliography}

% \input{reference}
% \newpage

% \end{document}
